# Supplementary material for: Improving Deep Policy Gradients with Value Function Search
Source: arXiv:2302.10145 source file (2023-02-20)
Supplement: Supplementary file 1 [file additional_statements.tex]

\section{Ethics Statement}

The proposed Value Function Search does not focus on experiments involving human subjects and does not require sensitive data that involve sex, gender, and diversity analysis. Hence, we do not consider the gender dimension, privacy, data governance issues, or any primary ethic concern highlighted in the \textit{ICLR Code of Ethics}\footnote{https://iclr.cc/public/CodeOfEthics} to be relevant.

However, according to the \textit{"Ethics Guidelines for Trustworthy Artificial Intelligence"} report published by the High-Level Expert Group on AI of the European Commission,\footnote{https://digital-strategy.ec.europa.eu/en/library/ethics-guidelines-trustworthy-ai} ethical consideration has to take into account the environment and the sustainability of AI systems.
Regarding the environmental impact, it is crucial to foster sample efficiency (i.e., reducing the training time for the agents, hence the computational resources used to train them) of Deep RL to lower energy consumption and related emissions. In this direction, VFS leads to significant benefits in sample efficiency, which reduces the environmental footprint of VFS-based approaches by a considerable margin.

In more detail, we employed the Machine Learning CO2 impact calculator \citep{CO2} to estimate the CO2 emissions of our experiments.\footnote{We note that this is not a precise measurement as it is not trivial to map energy consumption to CO2 emissions (i.e., the carbon footprint). To this end, we employed open-source electricity maps (e.g., https://www.electricitymaps.com) to estimate better how carbon-intensive our experiment's electricity is.} According to our hardware, the carbon efficiency of the provider, and the length of our experiments, we computed a total emission of $\approx 52.3$ kg CO2. We plan to cope with such emissions using Treedom\footnote{https://www.treedom.net}, an online service that allows us to plant trees to cope with our carbon footprint. 

\section{Reproducibility Statement}
Significant efforts have been made to ensure the reproducibility of VFS. Section 3 detail the flow of VFS-based algorithms with pseudocode and detailed explanations. We also highlight possible limitations of our approach in Section 3.1. Moreover, Section 4 states our experimental setup, while supplemental material contains a detailed overview of the considered hyperparameters.
